# Supplementary material for: RECAST: Approaching experimental accuracy in theoretical calculations of crystal structures
Source: arXiv:2611.39971 source file (2026-11-29)
Supplement: Supplementary file 2 [file si_tables.tex]

\newcommand{\tabpartcell}{42 & 1{,}794 & 4.10 & 0.86 & 0.93 & 0.65 & 0.67 & 1.42 & 0.43 & 0.11 & 0.07\\
43 & 1{,}794 & 4.10 & 0.89 & 0.93 & 0.64 & 0.68 & 1.43 & 0.44 & 0.11 & 0.08\\
44 & 1{,}792 & 4.16 & 0.86 & 0.94 & 0.65 & 0.68 & 1.45 & 0.43 & 0.11 & 0.07\\
45 & 1{,}796 & 4.10 & 0.83 & 0.93 & 0.64 & 0.66 & 1.41 & 0.42 & 0.11 & 0.08\\
46 & 1{,}787 & 4.21 & 0.87 & 0.96 & 0.65 & 0.69 & 1.45 & 0.43 & 0.11 & 0.08\\
47 & 1{,}795 & 4.05 & 0.79 & 0.92 & 0.65 & 0.67 & 1.41 & 0.41 & 0.11 & 0.08\\
48 & 1{,}796 & 4.13 & 0.82 & 0.94 & 0.64 & 0.66 & 1.43 & 0.42 & 0.11 & 0.08\\
49 & 1{,}797 & 4.12 & 0.86 & 0.96 & 0.65 & 0.68 & 1.44 & 0.43 & 0.11 & 0.08\\
50 & 1{,}794 & 4.12 & 0.86 & 0.94 & 0.65 & 0.67 & 1.42 & 0.42 & 0.11 & 0.08\\
51 & 1{,}792 & 4.13 & 0.84 & 0.89 & 0.62 & 0.65 & 1.42 & 0.41 & 0.11 & 0.08\\}
\newcommand{\tabpartatoms}{42 & 1.64 & 0.96 & 0.74 & 0.85 & 0.043 & 0.035 & 0.89 & 0.77\\
43 & 1.63 & 0.94 & 0.75 & 0.86 & 0.041 & 0.035 & 0.88 & 0.77\\
44 & 1.66 & 0.98 & 0.76 & 0.87 & 0.042 & 0.035 & 0.90 & 0.76\\
45 & 1.66 & 0.97 & 0.75 & 0.86 & 0.043 & 0.036 & 0.93 & 0.80\\
46 & 1.67 & 0.97 & 0.76 & 0.87 & 0.043 & 0.036 & 0.91 & 0.79\\
47 & 1.62 & 0.96 & 0.74 & 0.84 & 0.043 & 0.036 & 0.91 & 0.77\\
48 & 1.60 & 0.93 & 0.71 & 0.82 & 0.041 & 0.035 & 0.88 & 0.76\\
49 & 1.70 & 1.01 & 0.79 & 0.90 & 0.045 & 0.037 & 0.98 & 0.84\\
50 & 1.64 & 0.97 & 0.75 & 0.86 & 0.042 & 0.035 & 0.89 & 0.76\\
51 & 1.63 & 0.94 & 0.74 & 0.85 & 0.042 & 0.035 & 0.89 & 0.77\\}
\newcommand{\tabstrata}{$s_{\rm DFT}<1\%$ & 12{,}532 & 0.35 & 0.31 & 0.31 & 0.30 & 3.78 & 0.75 & 0.73 & 0.72 & 1.50 & 0.74\\
$1\leq s_{\rm DFT}<3\%$ & 4{,}308 & 1.68 & 1.08 & 1.04 & 1.03 & 4.81 & 1.01 & 0.96 & 0.95 & 1.84 & 0.98\\
$s_{\rm DFT}\geq3\%$ & 1{,}097 & 4.60 & 3.19 & 3.02 & 3.02 & 5.38 & 1.96 & 1.91 & 1.89 & 2.57 & 1.73\\
0D & 832 & 1.20 & 0.98 & 0.99 & 0.98 & 4.83 & 1.42 & 1.48 & 1.47 & 2.13 & 1.04\\
1D & 283 & 1.84 & 1.19 & 1.18 & 1.18 & 5.70 & 1.09 & 1.10 & 1.10 & 2.01 & 0.99\\
2D & 747 & 2.01 & 1.31 & 1.25 & 1.25 & 5.17 & 1.32 & 1.27 & 1.25 & 1.64 & 0.86\\
3D & 16{,}075 & 0.85 & 0.62 & 0.59 & 0.59 & 4.01 & 0.83 & 0.80 & 0.79 & 1.62 & 0.84\\
same space group & 17{,}511 & 0.93 & 0.67 & 0.65 & 0.64 & 4.13 & 0.88 & 0.86 & 0.85 & 1.64 & 0.85\\
space group differs & 426 & 1.01 & 0.73 & 0.72 & 0.71 & 3.93 & 1.03 & 0.98 & 0.98 & 1.72 & 1.01\\
high-pressure phase & 446 & 0.73 & 0.55 & 0.53 & 0.53 & 4.09 & 1.29 & 1.26 & 1.24 & 1.45 & 0.71\\
high- or low-$T$ phase & 507 & 1.00 & 0.74 & 0.73 & 0.73 & 4.13 & 1.22 & 1.21 & 1.21 & 1.79 & 1.16\\}
\newcommand{\tabsize}{1--4 & 1{,}507 & 3.29 & 1.39 & 0.50 & 0.43 & 1.21 & 0.61\\
5--8 & 2{,}117 & 3.22 & 0.95 & 1.05 & 0.74 & 1.46 & 0.83\\
9--16 & 3{,}133 & 3.93 & 0.83 & 1.07 & 0.70 & 1.65 & 0.91\\
17--32 & 4{,}339 & 4.31 & 0.77 & 1.02 & 0.70 & 1.69 & 0.87\\
33--64 & 4{,}298 & 4.61 & 0.74 & 0.95 & 0.65 & 1.75 & 0.86\\
65--200 & 2{,}543 & 4.47 & 0.78 & 0.74 & 0.52 & 1.78 & 0.91\\}
\newcommand{\tabcs}{1{,}132 & 4{,}419 & 4{,}581 & 2{,}417 & 1{,}468 & 1{,}517 & 2{,}522}
