# Supplementary material for: RECAST: Approaching experimental accuracy in theoretical calculations of crystal structures
Source: arXiv:2611.39971 source file (2026-11-29)
Supplement: Supplementary file 3 [file si_tables_extra.tex]

\newcommand{\tabstratablocks}{\multicolumn{12}{@{}l}{\emph{DFT shape error}}\\
$s_{\rm DFT}<1\%$ & 12{,}532 & 0.35 & 0.31 & 0.31 & 0.30 & 3.78 & 0.75 & 0.73 & 0.72 & 1.50 & 0.74\\
$1\leq s_{\rm DFT}<3\%$ & 4{,}308 & 1.68 & 1.08 & 1.04 & 1.03 & 4.81 & 1.01 & 0.96 & 0.95 & 1.84 & 0.98\\
$s_{\rm DFT}\geq3\%$ & 1{,}097 & 4.60 & 3.19 & 3.02 & 3.02 & 5.38 & 1.96 & 1.91 & 1.89 & 2.57 & 1.73\\
\addlinespace
\multicolumn{12}{@{}l}{\emph{Dimensionality of the bonded network}}\\
0D & 832 & 1.20 & 0.98 & 0.99 & 0.98 & 4.83 & 1.42 & 1.48 & 1.47 & 2.13 & 1.04\\
1D & 283 & 1.84 & 1.19 & 1.18 & 1.18 & 5.70 & 1.09 & 1.10 & 1.10 & 2.01 & 0.99\\
2D & 747 & 2.01 & 1.31 & 1.25 & 1.25 & 5.17 & 1.32 & 1.27 & 1.25 & 1.64 & 0.86\\
3D & 16{,}075 & 0.85 & 0.62 & 0.59 & 0.59 & 4.01 & 0.83 & 0.80 & 0.79 & 1.62 & 0.84\\
\addlinespace
\multicolumn{12}{@{}l}{\emph{Space group}}\\
same space group & 17{,}511 & 0.93 & 0.67 & 0.65 & 0.64 & 4.13 & 0.88 & 0.86 & 0.85 & 1.64 & 0.85\\
space group differs & 426 & 1.01 & 0.73 & 0.72 & 0.71 & 3.93 & 1.03 & 0.98 & 0.98 & 1.72 & 1.01\\
\addlinespace
\multicolumn{12}{@{}l}{\emph{Phase}}\\
high-pressure phase & 446 & 0.73 & 0.55 & 0.53 & 0.53 & 4.09 & 1.29 & 1.26 & 1.24 & 1.45 & 0.71\\
high- or low-$T$ phase & 507 & 1.00 & 0.74 & 0.73 & 0.73 & 4.13 & 1.22 & 1.21 & 1.21 & 1.79 & 1.16\\
\addlinespace
\multicolumn{12}{@{}l}{\emph{Functional}}\\
DFT & 14{,}701 & 0.91 & 0.66 & 0.64 & 0.64 & 3.96 & 0.90 & 0.88 & 0.87 & 1.57 & 0.83\\
DFT+$U$ & 3{,}236 & 1.02 & 0.71 & 0.68 & 0.67 & 4.87 & 0.81 & 0.77 & 0.76 & 1.96 & 0.98\\
\addlinespace
\multicolumn{12}{@{}l}{\emph{Atoms in the cell}}\\
1--4 & 1{,}507 & 0.50 & 0.40 & 0.44 & 0.43 & 3.29 & 1.40 & 1.42 & 1.39 & 1.21 & 0.61\\
5--8 & 2{,}117 & 1.05 & 0.78 & 0.75 & 0.74 & 3.22 & 0.97 & 0.96 & 0.95 & 1.46 & 0.83\\
9--16 & 3{,}133 & 1.07 & 0.75 & 0.71 & 0.70 & 3.93 & 0.88 & 0.84 & 0.83 & 1.65 & 0.91\\
17--32 & 4{,}339 & 1.02 & 0.73 & 0.70 & 0.70 & 4.31 & 0.81 & 0.78 & 0.77 & 1.69 & 0.87\\
33--64 & 4{,}298 & 0.95 & 0.67 & 0.65 & 0.65 & 4.61 & 0.79 & 0.75 & 0.74 & 1.75 & 0.86\\
65--200 & 2{,}543 & 0.74 & 0.54 & 0.53 & 0.52 & 4.47 & 0.82 & 0.78 & 0.78 & 1.78 & 0.91\\}
\newcommand{\tabsimple}{constant correction & 17{,}937 & 4.12 & 2.08 & 0.85 & 0.93 & 0.93 & 0.64\\
hydrostatic pressure & 16{,}354 & 4.02 & 0.00 & 0.79 & 0.87 & 1.07 & 0.60\\
relaxation with D3 & 17{,}712 & 4.11 & 2.92 & 0.84 & 0.93 & 1.28 & 0.64\\
relaxation without D3 & 17{,}570 & 4.09 & 5.16 & 0.83 & 0.93 & 1.63 & 0.64\\}
\newcommand{\tabrefAsi}{all five, three initializations each (the correction) & 15 & 0.85 & 0.64 & 0.42 & 0.08 & 0.86\\
all five, one initialization each & 5 & 0.86 & 0.65 & 0.43 & 0.08 & 0.86\\
direct strain head, three initializations & 3 & 0.92 & 0.71 & 0.46 & 0.09 & 0.87\\
direct strain head, five initializations & 5 & 0.91 & 0.70 & 0.46 & 0.09 & 0.87\\
estimator 5, three initializations & 3 & 0.88 & 0.65 & 0.43 & 0.08 & 0.86\\
estimator 5, five initializations & 5 & 0.87 & 0.65 & 0.43 & 0.08 & 0.86\\
estimators 1--3, three initializations each & 9 & 0.86 & 0.66 & 0.43 & 0.08 & 0.86\\
estimators 4--5, three initializations each & 6 & 0.87 & 0.65 & 0.43 & 0.08 & 0.86\\
estimator 2, three initializations & 3 & 0.90 & 0.71 & 0.46 & 0.09 & 0.87\\
estimator 3, three initializations & 3 & 0.88 & 0.68 & 0.45 & 0.08 & 0.87\\
estimator 4, three initializations & 3 & 0.88 & 0.67 & 0.44 & 0.08 & 0.86\\}
\newcommand{\Nreserved}{4{,}659}
\newcommand{\Neligible}{13{,}397}
